# Supplementary material for: Resource theories of knowledge
Source: arXiv:1511.08818 source file (2015-11-27)
Supplement: Supplementary file 1 [file appendix_applications.tex]

\begin{bigexample}{Memories in traditional resource theories}{memories}

\lea{One could leave this paragraph out and leave out the B system, drawing the arrow only on SM. I am not so sure how clear it will be then though.} Consider a resource theory of quantum states and thermal operations, in which the total Hilbert space is given by $\hilbert_S\otimes\hilbert_M\otimes\hilbert_R\otimes\hilbert_B$, where $S$, $M$, $R$ and $B$ denote the target system, memory, reference systems (which the agent cannot access) and thermal bath systems respectively. The total Hamiltonian is $H=H_S\otimes \id_{MRB} + H_M\otimes \id_{SRB} + H_R\otimes\id_{SMB} + H_B\otimes\id_{SMR}$, and the bath states are Gibbs states $\tau_B$ at temperature $T$. The allowed operations are energy-preserving unitary operations $U_{SMB}$ on systems $S$, $M$ and $B$.

Now, for the use of the memory within such a resource theory, we would demand that the local states on memory and reference systems be preserved. We would then say that a transformation $\rho \to \sigma$ \emph{acts on $S$, using $M$ as a memory} and $R$ as a reference if
\begin{align*}
\rho_{SMR}\otimes\tau_B \stackrel{S M B}{\longrightarrow} \sigma_{SMRB} 
\quad \text{and} \quad 
\rho_{M R} = \sigma_{M  R}.
\end{align*}

where $\stackrel{S M B}{\longrightarrow}$ here denotes that there exists an allowed operation in $SMB$ that achieves the transformation.

A paradigmatic example of such a process is the erasure of a subsystem, which might be correlated with a memory (a classical example is the formatting of a disk). The study of erasure gave rise to Landauer's principle, the key connection between thermodynamics and information theory, and helped solve puzzles like Maxwell's demon and Gibbs' paradox. \lea{cite some stuff?}

In the resource theory of quantum thermal operations as above, let $\ket{0}_S$ be a fixed, extremal local state in $\hilbert_S$. Erasure of system $S$ (assisted by memory $M$) is then a process
\begin{align*}
\rho_{SMR}\otimes \tau_B \stackrel{SMB}{\longrightarrow} 
\ket{0}\bra{0}_S \otimes \rho_{MR}
\end{align*}
which uses $M$ as a memory.

To see how these definitions fit into our generalized notion, note that the traditional subsystems are in our definition replaced by the embedding $\e_M$, which would correspond to a local state in the memory. The condition that the state of the memory is preserved is naturally taken over and phrased in terms of such a (local) embedding. Here, we need not distinguish between the systems $M$ and $R$ and the embedding $\e_M$ would essentially include both systems. The actual distinction between the memory and the reference arises through the functions the agent is allowed to implement, which we assume to already feature in the agent's resource theory. That is, $\to$ in our generalized framework already includes the information which systems are accessible to the agent.
\end{bigexample}
