# Supplementary material for: Resource theories of knowledge
Source: arXiv:1511.08818 source file (2015-11-27)
Supplement: Supplementary file 2 [file appendix_copies.tex]

Here we build up the notion of copies of a local specification. First we need to establish what it means for two subsystems to be identical, and what it means to permute them.

\subsection{Swaps and permutations}

\begin{definition}[Identical subsystems]
Let $(S^\Omega, \cT)$ be a resource theory. We say that two  submonoids of transformations $A,B \subseteq \cT$ are \emph{identical} if they are isomorphic. 

Let $i: A \to B$ be an isomorphism between two identical systems $A$ and $B$, and let $f_A\in A, g_B \in B$. We denote 
\begin{align*}
  f_B &:= i(f_A),\\
  g_A &:= i^{-1}(g_B).
\end{align*}
In the following we will make the isomorphism $i$ implicit.

\end{definition}

%\begin{remark}
%Let $(S^\Omega, \cT)$ be a resource theory. If two complete independent systems $A$ and $B$ are identical, then the local specification spaces $S^{\Omega_A}$ and $S^{\Omega_B} $ generated by the monoids $A$ and $B$ (as in Theorem \ref{thm:transformations_independent_agents}) are isomorphic.
%\end{remark}

We define the remaining concepts in this section for complete subsystems ($\bic A = A$). They could possibly be generalized to other submonoids of transformations (associated with local agents). 

\begin{definition}[Swaps]
Let $(S^\Omega, \cT)$ be a resource theory, and let $A$ and $B$ be two complete independent and identical subsystems. We say that a pair of functions $(u_{AB}, u'_{AB}) \in (A\vee B)^{\times 2}$ \emph{swap} $A$ and $B$ if
\begin{align*}
  u'_{AB}\ f_A\ g_B\ u_{AB} 
  &= u_{AB}\ f_A\ g_B\ u'_{AB} 
  = f_B\ g_A,
\end{align*}
for all $f_A\in A, g_B \in B$.

We say that two identical, independent subsystems $A$ and $A'$ \emph{may swap} if there exists a swap $(u_{AA'}, u'_{AA'}) \in (A \vee A')^{\times 2}$ between them. 
%For any subsystem $A$ in a resource theory $(S^\Omega, \cT)$ we denote by $\mathcal A$  the set of all the subsystems that may swap with $A$, plus $A$. 
\end{definition}

For example, take a resource theory of local operations between two parties, Alice and Bob.  Then all identical and independent subsystems of Alice's system are swappable, and the same for Bob. We are not allowed, however, to swap subsystems between Alice and Bob.

\begin{remark}
Note that, in particular, because the identity transformation $1 \in A, B$,
\begin{align*}
  & u'_{AB}\ 1 \circ 1  \ u_{AB} =  u_{AB}\ 1 \circ 1 \ u'_{AB} = 1 \circ 1
  \quad \Leftrightarrow \\
  \Leftrightarrow\quad & u'_{AB}\ u_{AB}= u_{AB}\ u'_{AB} = 1.
\end{align*}
In other words, $u_{AB}$ is invertible (a reversible operation), and its inverse is $u'_{AB} =: u^{-1}_{AB}$.

From now on, we will say that $u_{AB} \in A \vee B$ swaps $A$ and $B$, and call it a subsystem swap, if it is invertible and $(u_{AB}, u^{-1}_{AB})$ swap $A$ and $B$. 
\end{remark}

\begin{remark}
Let $(S^\Omega,\cT)$ be a resource theory. Since any swap $u_{AB}\in\cT$ is an invertible endomorphism and thus injective, $u_{AB}(\Omega)=\Omega$.
\end{remark}

\begin{proposition}
Let $(S^\Omega,\cT)$ be a resource theory, $A$ and $B$ swappable subsystems in $\cT$ with swap $u_{AB}$. 
Let $\Lump$ be a lumping in $S^\Omega$ inducing an intensive embedding $(\e, \h)$ of a specification space $S^\Gamma$  in $S^\Omega$ that is independent of $A$.  Then $\Lump':=u'_{AB}\circ\Lump\circ u_{AB}$ is again a lumping inducing  an intensive embedding $(\e', \h')$ of a specification space $S^\Sigma$  in $S^\Omega$ that is independent of $B$. 
\end{proposition}

\begin{proof}
The function $$\Lump':=u'_{AB}\circ\Lump\circ u_{AB}$$ is  idempotent and inflating since $\Lump$ is. It also automatically satisfies for all $f_B\in B$
\begin{align*}
\Lump'\circ f_B&=u'_{AB}\circ\Lump\circ u_{AB}\circ f_B\\
&=u'_{AB}\circ\Lump\circ u_{AB}\circ f_B\circ u'_{AB}\circ u_{AB}\\
&=u'_{AB}\circ\Lump\circ f_A\circ u_{AB}\\
&=u'_{AB}\circ\Lump\circ u_{AB}\\
&=\Lump'
\end{align*}
since $f_A\in A$ and $\Lump$ is independent of $A$.
\end{proof}

\begin{proposition}
Let $(S^\Omega,\cT)$ be a resource theory, $A$ and $B$ isomorphic subsystems in $\cT$ swappable with $u_{AB}$ and $\Lump_{\cancel A}$ be the lumping generated by $A$, 
$\Lump_{\cancel A} (V) = \bigcup_{f_A \in A} \{W: f_A(W) = f_A(V)\}$. Then $u'_{AB}\circ\Lump_{\cancel A}\circ u_{AB} = \Lump_{\cancel B}$.
\end{proposition}

\begin{proof}
We have
\begin{align*}
u^{-1}_{AB}\circ\Lump_{\cancel A}\circ u_{AB}(V)
&=\bigcup_{f_A\in A}\{u^{-1}_{AB} (W):f_A(W)=f_A \circ u_{AB}(V)\}\\
&= \bigcup_{f_A\in A}\{u^{-1}_{AB} (W):f_A \circ \underbrace{u_{AB} \circ u^{-1}_{AB}}_{\flag{1}} (W)=f_A \circ u_{AB}(V)\}\\
\flag{u_{AB}\text{ reversible}}&=   \bigcup_{f_A\in A}\{u^{-1}_{AB} (W): u^{-1}_{AB} \circ f_A \circ u_{AB} \circ u^{-1}_{AB} (W)= u^{-1}_{AB} \circ f_A \circ u_{AB}(V)\}\\
&= \bigcup_{f_A\in A}\{u^{-1}_{AB} (W):  f_B  \circ u^{-1}_{AB} (W)=  f_B (V)\}\\
&= \bigcup_{f_B\in B}\{W':  f_B   (W')=  f_B (V)\}\\
&= \Lump_{\cancel B} (V).
\end{align*}
\end{proof}

%\begin{corollary}
%The lumpings associated 
%\end{corollary}

\begin{definition}[Permutations of specifications]
Let $(S^\Omega, \cT)$ be a resource theory. Let $A$ be a subsystem and $V$  a specification. 
We say that a specification $V'$ is a \emph{permutation} of $V$ if  
\begin{align*}
\exists A'\in \mathcal A: \ V'= u_{AA'}(V),
\end{align*}
where $u_{AA'}$ is a swap from $A$ to $A'$.

We say that a specification $V$ is \emph{permutation-invariant} over a collection $\mathcal{A}$ of identical subsystems if for all $A,A'\in\mathcal{A}$, $V=u_{AA'}(V)$.

\end{definition}

\subsection{Copies of resources}

\begin{definition}[Identical agents and copies]
Let $(S^\Omega, \cT)$ be a resource theory, and let $(S^A,\tilde A)$ and $(S^B,\tilde B)$ be two independent restricted resource theories arising from two identical, swappable subsystems $A,B\in\Sys(\cT)$. Then we say that $(S^B,\tilde B)$ is an \emph{independent copy} of $(S^A,\tilde A)$. %\flag{why are we defining this at the level of agents?}

If $\local{V_A}$ is a local specification in $S^A$, we say that $\local{V_B}:=u_{AB}(\local{V_A})$ is a \emph{copy} of $\local{V_A}$ from $(S^A,\tilde A)$ in $(S^B,\tilde B)$. 
%In this case, we denote by $\Cop(V)_{A}$ the set of all copies of $[V]_A$,
%$$ 
%\Cop([V]_A) = \{ [V]_{A'} =  u_{AA'}([V]_A), \ A'\in \mathcal A \}.
%$$
\end{definition}

\begin{remark}
A copy $V_B=u_{AB}(\local{V_A})$ is indeed local in $S^B$, that is, $\Lump_B(\local{V_B})=\local{V_B}$.
\end{remark}
\begin{proof}
Follows directly by substituting $\Lump_B=u_{AB}\circ \Lump_A\circ u^{-1}_{AB}$ and using that $\local{V_A}$ is local in $S^A$.
\end{proof}

\begin{proposition}
Let $(S^{\Omega}, \cT)$ be a resource theory, and let $A,B\in\Sys(\cT)$ be two independent and identical subsystems. If for all $V,W\in S^{\Omega}$ $$\exists X\in S^\Omega,f_A\in A,f_B\in B \text{ s.t. } f_A(V)=f_A(X), f_B(W)=f_B(X)$$
then the 
local descriptions induced by $\Lump_{\cancel A} $ and $\Lump_{\cancel B}$ are freely composable. Furthermore, the corresponding
restricted resource theories  (with transformations $\tilde B$ and $\tilde A$ respectively) are independent. 
\end{proposition}

\begin{proof}
% did we prove that they are freely composable? check!
By construction, the space induced by $\Lump_{\cancel A}$ is independent of $A$ and vice versa for $B$. Now, it is left to show that $\Lump_{\cancel A}\circ\Lump_{\cancel B}(V)=\Omega$ for all $V\in S^\Omega$. We have
\begin{align*}
\Lump_{\cancel A}\circ\Lump_{\cancel B}(V)&=\Lump_A\left(\bigcup_{X\in S^\Omega,f_B\in B}(X: f_B(X)=f_B(V))\right)\\
&=\bigcup_{Y\in S^\Omega}\bigcup_{X\in S^\Omega}\bigcup_{f_A\in A,f_B\in B}(Y: f_A(Y)=f_A(X),f_B(X)=f_B(V))\\
&=\Omega,
\end{align*}
and so the local descriptions are freely composable.
\end{proof}

\begin{definition}[Copies of specifications]
Let $(S^\Omega, \cT)$ be a resource theory, $A$ be a subsystem and let $\text{\AA}_n \subseteq \mathcal A$ be a set $n$ of mutually independent, swappable copies of $A$.\footnote{Pronounced as in {\AA}berg.} Let $(S^A,\tilde A)$ be a restricted resource theory arising from $A$, and let $\{(S^{A_i},\tilde A_i)\}_i$ be a set of $n$ independent copies of $(S^A,\tilde A)$ belonging to $\text{\AA}_n$.  Finally, let  $\local{V_A}$ be a local specification in $A$. 
We denote the specification of $n$ \emph{copies} of $V_A$ in $\text{\AA}_n$ by
$$V_A^{n} :=  \bigcap_{A'\in \text{\AA}_n} u_{AA'}(\local{V_A}) \quad \in S^\Omega.$$
Often we will make the set $\text{\AA}_n$ implicit, and call it simply the \emph{support} of the copies. 
%\footnote{After all, \AA \ is shy.} 
We define taking zero copies of any resource as the trivial specification, $V_A^{0}:=\Omega$.
\end{definition}
% xxxxxxxxxxxxxxxxxxxxxxxxxx
% xxxxxxxxxxxxxxxxxxxxxxxxxx

%\begin{remark}
%$V_A^{\otimes n}$ is local in $\bigvee_{A'\in \AA_n} A'$, which is why we call $\AA_n$ its support.
%\end{remark}

\begin{example}[Copies of pure qubits]

%
%
%Consider the setting of unital operations. $\Omega$ is the set of density operators over a large but finite Hilbert space, and $\cT$ is the set of all unital maps in that space. Then $(S^\Omega, \cT)$ inherits a strong local structure and a well-defined notion of uncorrelated systems from quantum theory.

Consider quantum theory, and the specification $[\ket0]_A$, which represents the knowledge `qubit $A$ is in pure state $\ket0$', $\local{\ket0_A}= \{\omega \in \Omega: \tr_{\com A} \omega= \pure0_A \}$. The set of local operations in qubit $A$ form a subsystem $A$, and $\local{\ket0_A}$ is a local specification in the embedding given by $\tr_{\com A}$.

By combining $n$ copies of $\local{\ket0_A}$ we obtain the description of $n$ pure qubits. For instance, for $\text \AA = \{A, A'\}$,
 \begin{align*}
  \ket0_A^{2} 
  &= \local{\ket0_A} \ \cap\ u_{AA'}(\local{\ket0_{A}})  \\
  &=  
   \{\omega \in \Omega: \ \tr_{\com{A}}(\omega) = \pure{0} \} 
   \cap 
   \{\omega \in \Omega: \ \tr_{\com{A'}}(\omega) = \pure{0} \}  \\
   &=\{\omega \in \Omega: \ \tr_{\com{AA'}}(\omega) = \pure{00} \} \\
   &= \local{\ket{00}_{AA'}}.
 \end{align*}
\end{example}
